# Supplementary material for: Practical sensorless aberration estimation for 3D microscopy with deep learning
Source: arXiv:2006.01804 ancillary file (2020-07-05)
Supplement: Supplementary file 1 [file supplement.pdf]

# Practical sensorless aberration estimation for 3D microscopy with deep learning

DEBAYAN SAHA<sup>1,2</sup>, UWE SCHMIDT<sup>1,2</sup>, QINRONG ZHANG<sup>3</sup>, AURELIEN BARBOTIN<sup>4</sup>,  
 QI HU<sup>4</sup>, NA JI<sup>3</sup>, MARTIN J. BOOTH<sup>4,\*</sup>, MARTIN WEIGERT<sup>1,2,5,\*</sup>, AND EUGENE W.  
 MYERS<sup>1,2,\*</sup>

<sup>1</sup>MPI-CBG, Dresden, Germany

<sup>2</sup>CSBD, Dresden, Germany

<sup>3</sup>University of California, Berkeley, USA

<sup>4</sup>University of Oxford, Department of Engineering Science, Oxford, UK

<sup>5</sup>Institute of Bioengineering, School of Life Sciences, EPFL, Lausanne, Switzerland

\*Corresponding author: myers@mpi-cbg.de, martin.weigert@epfl.ch, martin.booth@eng.ox.ac.uk

Compiled July 5, 2020

Estimation of optical aberrations from volumetric intensity images is a key step in sensorless adaptive optics for 3D microscopy. Recent approaches based on deep learning promise accurate results at fast processing speeds. However, collecting ground truth microscopy data for training the network is typically very difficult or even impossible thereby limiting this approach in practice. Here, we demonstrate that neural networks trained *only* on *simulated* data yield accurate predictions for *real* experimental images. We validate our approach on simulated *and* experimental datasets acquired with two different microscopy modalities, and also compare the results to non-learned methods. Additionally, we study the predictability of individual aberrations with respect to their data requirements and find that the symmetry of the wavefront plays a crucial role. Finally, we make our implementation freely available as open source software in Python.

© 2020 Optical Society of America under the terms of the [OSA Open Access Publishing Agreement](#)

<http://dx.doi.org/10.1364/optica.XX.XXXXXX>

## CONTENTS

|   |                                   |   |
|---|-----------------------------------|---|
| 1 | Supplementary Notes               | 2 |
| A | Classical Methods . . . . .       | 2 |
| B | Multi-plane experiments . . . . . | 2 |
| 2 | Supplementary Tables              | 2 |
| 3 | Supplementary Figures             | 2 |

## 1. SUPPLEMENTARY NOTES

### A. Classical Methods

**Gerchberg-Saxton GS** We use an already published modified GS implementation (made available to us by the authors from [1]) and adapted it to the images from the experimental data sets (e.g. input image sizes). We checked the validity of the code by applying it to noise-free synthetic images, where the resulting wavefront was in good agreement to the ground-truth wavefront. Slightly better performance of GS was noticed on masking the periphery of the pupil plane, however the results are not shown here.

**ZOLA** We used the ZOLA plugin (<https://github.com/imodpasteur/ZOLA-3D>) available for ImageJ/Fiji [2, 3]. We wrote a macro in Fiji that loads the 3D image, automatically selects the pixel of maximal intensity, and calls the Zola plugin. The physical parameters of Zola were set according to the respective microscope setup. Good performance was obtained from the default camera parameters so they were not changed. We used 30 iteration steps for the optimization with GPU acceleration activated (NVIDIA Titan Xp). From the predicted amplitudes  $a_i$  we extracted the first 15 Zernike mode amplitudes, and converted them to Noll order omitting  $a_1, a_2, a_3, a_4$  (piston, tip, tilt, defocus).

### B. Multi-plane experiments

**Training data** We first generated isotropic 3D synthetic PSFs according to the microscope parameters with a fixed number of planes  $n_{z0} = 64$ . From these we created smaller images with  $n_z$  planes by taking the  $\pm 2k$ -th plane from either side of the middle plane ( $k = 0 \dots n_x/2$ ).

**Experimental data** From the 3D bead images acquired for single mode and random mode experiments (POINT SCANNING and WIDEFIELD), we took the maximum intensity plane as the mid plane and cropped the images as described above.

**RMSE calculation for odd/even modes experiment** We reconstruct the wavefront for both PHASENET predictions and ground truth as a weighted sum of Zernike modes defined on the back pupil as described above. We then grouped both wavefronts into their even and odd components and computed the RMSE between predicted and ground truth component separately.

## 2. SUPPLEMENTARY TABLES

| Method   | single ( $n = 1$ ) | batched ( $n = 50$ ) |
|----------|--------------------|----------------------|
| GS       | 0.12s              | 6.2s                 |
| Zola     | 17.1s              | 838s                 |
| PHASENET | 4ms                | 33ms                 |

**Table S1.** Runtime of all methods for aberration estimation from a single ( $n = 1$ ) and multiple ( $n = 50$ ) PSFs of size  $32 \times 32 \times 32$ .

| Method   | single ( $n = 1$ ) | batched ( $n = 50$ ) |
|----------|--------------------|----------------------|
| GS       | 0.98s              | 49s                  |
| Zola     | 28s                | 1475s                |
| PHASENET | 5ms                | 110ms                |

**Table S2.** Runtime of all methods for aberration estimation from a single ( $n = 1$ ) and multiple ( $n = 50$ ) PSFs of size  $50 \times 50 \times 50$ .

## 3. SUPPLEMENTARY FIGURES

### REFERENCES

1. P. Kner, L. Winoto, D. A. Agard, and J. W. Sedat, "Closed loop adaptive optics for microscopy without a wave-front sensor," in *Three-Dimensional and Multidimensional Microscopy: Image Acquisition and Processing XVII*, vol. 7570 (International Society for Optics and Photonics, 2010), p. 757006.
2. J. Schindelin, I. Arganda-Carreras, E. Frise, V. Kaynig, M. Longair, T. Pietzsch, S. Preibisch, C. Rueden, S. Saalfeld, B. Schmid *et al.*, "Fiji: an open-source platform for biological-image analysis," *Nat. methods* **9**, 676–682 (2012).
3. C. A. Schneider, W. S. Rasband, and K. W. Eliceiri, "Nih image to imagej: 25 years of image analysis," *Nat. methods* **9**, 671–675 (2012).
4. A. Barbotin, S. Galiani, I. Urbančič, C. Eggeling, and M. J. Booth, "Adaptive optics allows sted-fcs measurements in the cytoplasm of living cells," *Opt. express* **27**, 23378–23395 (2019).

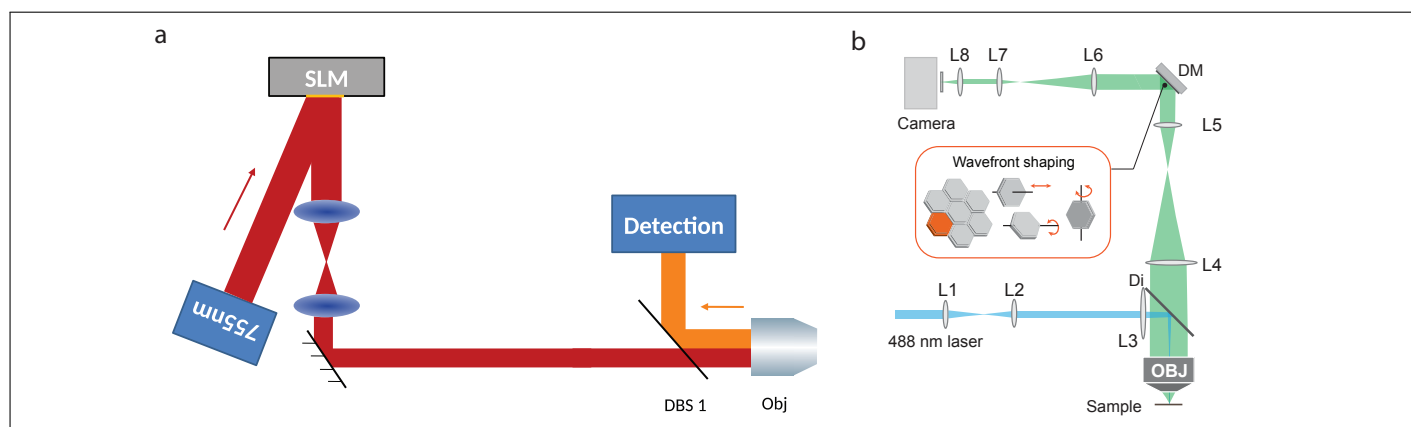

**Fig. S1.** Schematics of microscope set-ups. a) Adaptive point scanning microscope built around the modified, commercial RESOLFT microscope (Abberior Instruments, Germany). A  $755\text{nm}$  laser (blue box with red beam path) was focused by a  $100\times/1.4$  oil immersion objective (Obj; Olympus UPLSAPO). The phase of the laser was spatially modulated using a spatial light modulator (SLM; Hamamatsu LCOS X10468-02) which was relayed to the back focal plane of the objective using a pair of lenses (blue ellipses). The scattered light from a gold bead at focus of the objective was separated from the excitation light using a dichroic beam splitters (DBS 1) and was collected using a photomultiplier tube (blue box, Detection). (Figure reproduced with permission from [4], Creative Commons license CC BY 4.0). b) Home-built widefield fluorescence microscope. The output beam from a  $488\text{-nm}$  continuous laser (blue beam path) was expanded to  $8.4\text{ mm}$  in diameter before entering the microscope. And the beam was de-magnified to the sample plane by three lenses ( $L1, L2, L3$ ) and a  $25\times/1.1$  water immersion objective lens (OBJ; Nikon, CFI Apo LWD). A dichroic mirror (Di) was placed between  $L3$  and the objective, reflecting illumination and transmitting emitted fluorescence. Emitted fluorescence (green beam path) was collected with the same objective, whose back focal plane was relayed to the deformable mirror (DM; Iris AO, PTT489) by a pair of lenses ( $L4$ - $L5$ ). The DM-reflected fluorescence was then focused and imaged on the camera by 3 lenses ( $L6$ - $L7$ - $L8$ )

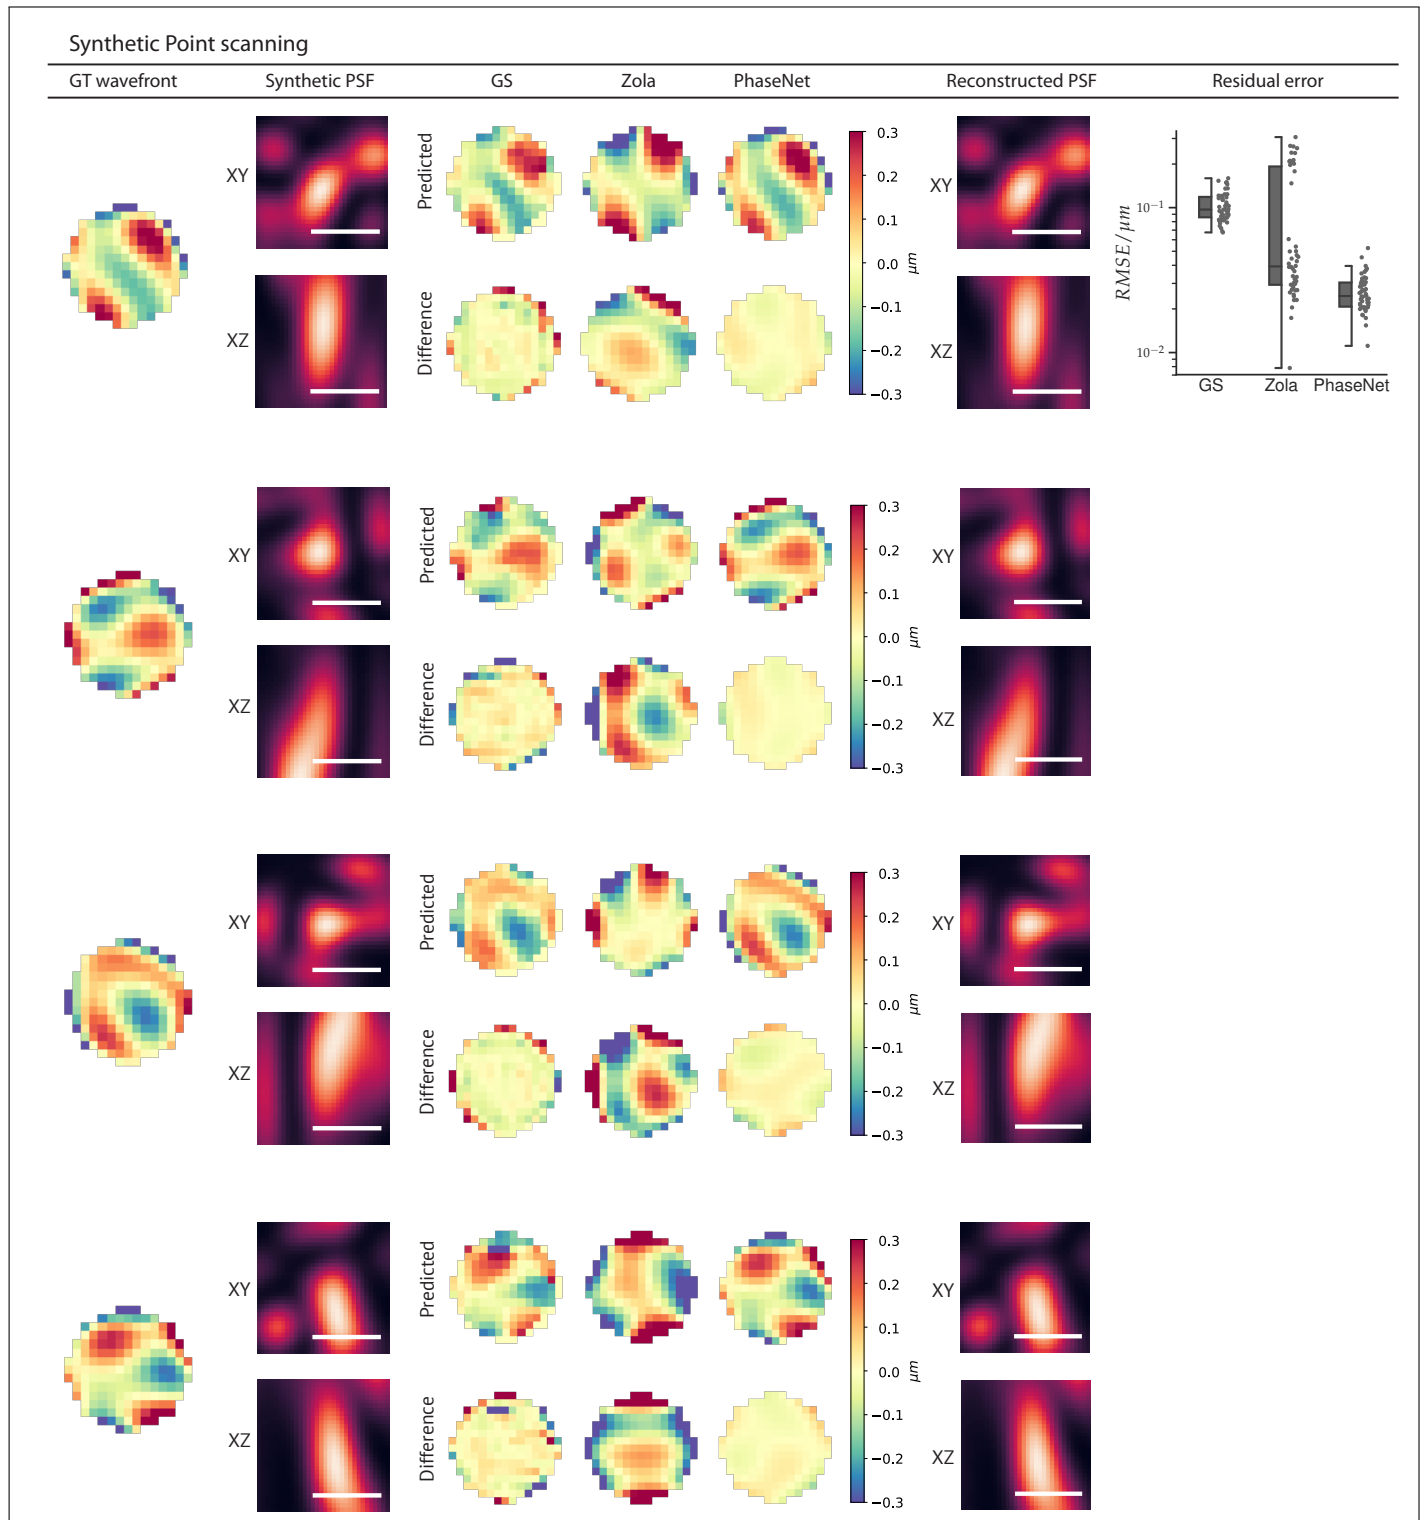

**Fig. S2.** Results on synthetic data. Random amplitudes of Zernike modes (Noll 5-15) in the range  $[-0.075, 0.075]\mu\text{m}$  for each mode was used to create GT wavefronts. The corresponding 3D intensity PSFs were simulated, convolved with a sphere of  $100\text{nm}$  diameter and noise was added to create 3D synthetic PSFs. We cropped the PSFs to an isotropic volume of 32 planes and  $(32 \times 32)$  pixels to match the input shape of the network. Here we show examples of the ground truth wavefronts (reconstructed from the amplitudes of Zernike coefficients), lateral (XY) and axial (XZ) midplanes of the synthetic PSFs, the wavefronts estimated with Gerchberg-Saxton, Zola, and PHASENET (upper row) and their difference from the ground truth wavefronts (lower row), and the reconstructed PSFs from the PHASENET predictions. Additionally we show for all methods the error of the predicted wavefronts (root mean square error, RMSE) for 50 synthetic PSFs. Scalebar:  $500\text{nm}$ .

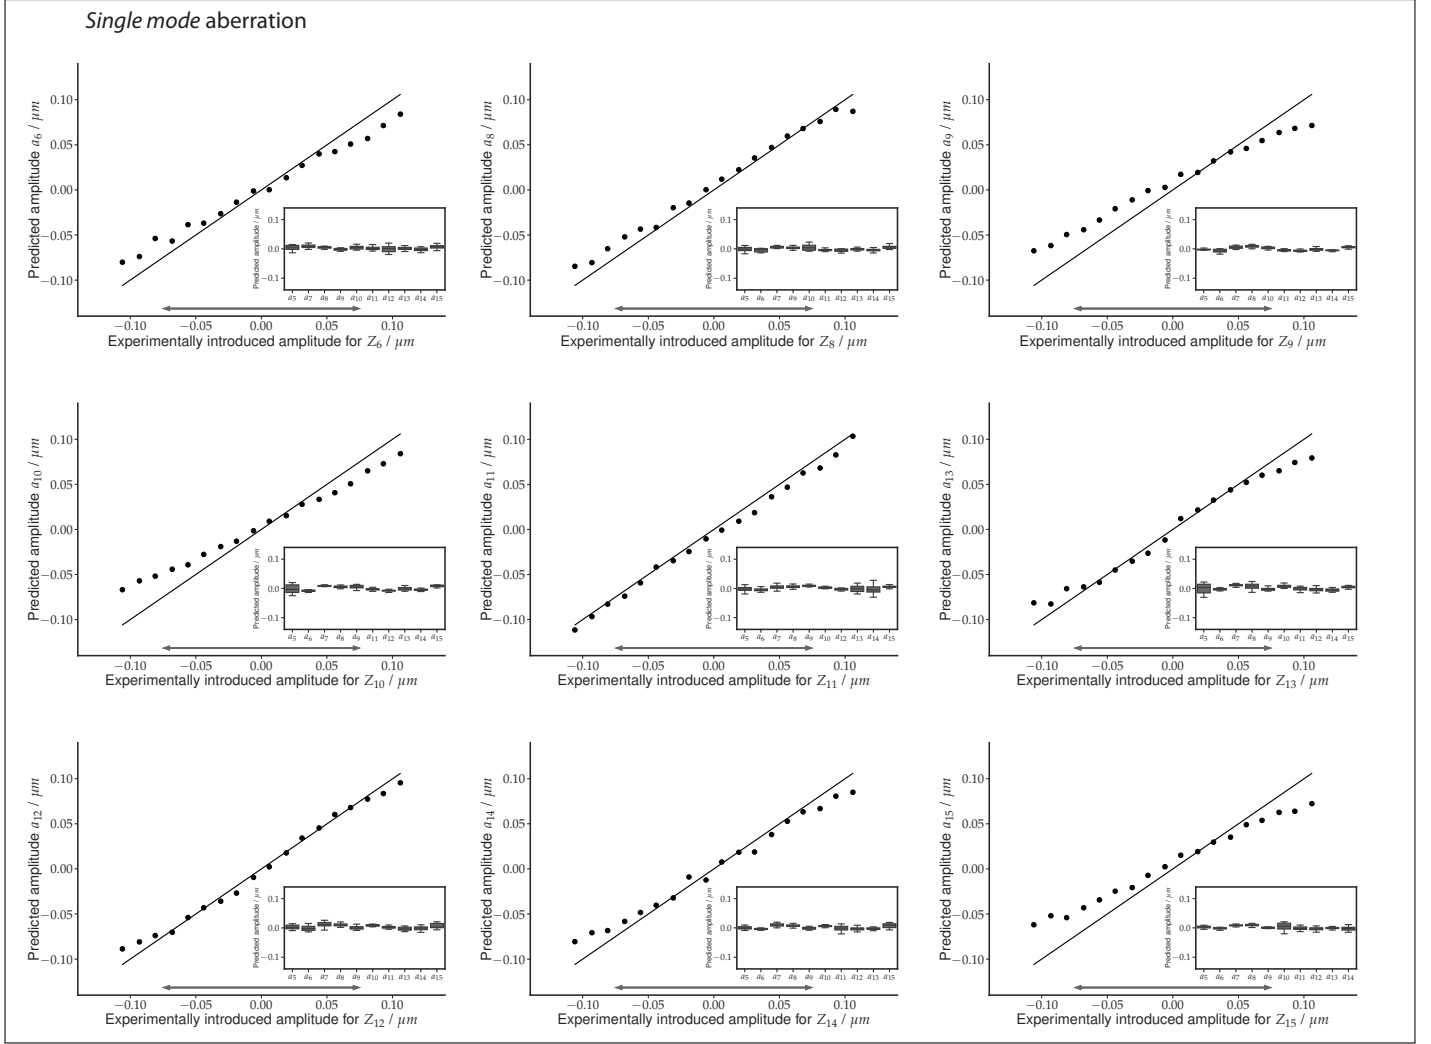

**Fig. S3.** Results of PHASENET on experimental *single mode* aberrations. A spatial light modulator was used to introduce single mode aberrations in the range  $[-0.11, 0.11] \mu\text{m}$  and the respective 3D stacks ( $n_z = 32$  planes) of 80 nm gold beads were acquired. A network trained on synthetic PSFs was used for predicting aberration amplitudes ( $a_5, \dots, a_{15}$ ) from the 3D stacks. Each graph shows the predicted amplitude for the single experimentally introduced Zernike mode *vs.* the ground truth amplitude of that mode for each single mode experiment. The inset of each graph depicts the distribution of predictions for the remaining non-introduced modes for that experiment. The solid black line of unit slope indicates perfect prediction, the gray arrow depicts the upper and lower bound of amplitudes for which the network was trained ( $a_i \in [-0.075, 0.075] \mu\text{m}$ ).

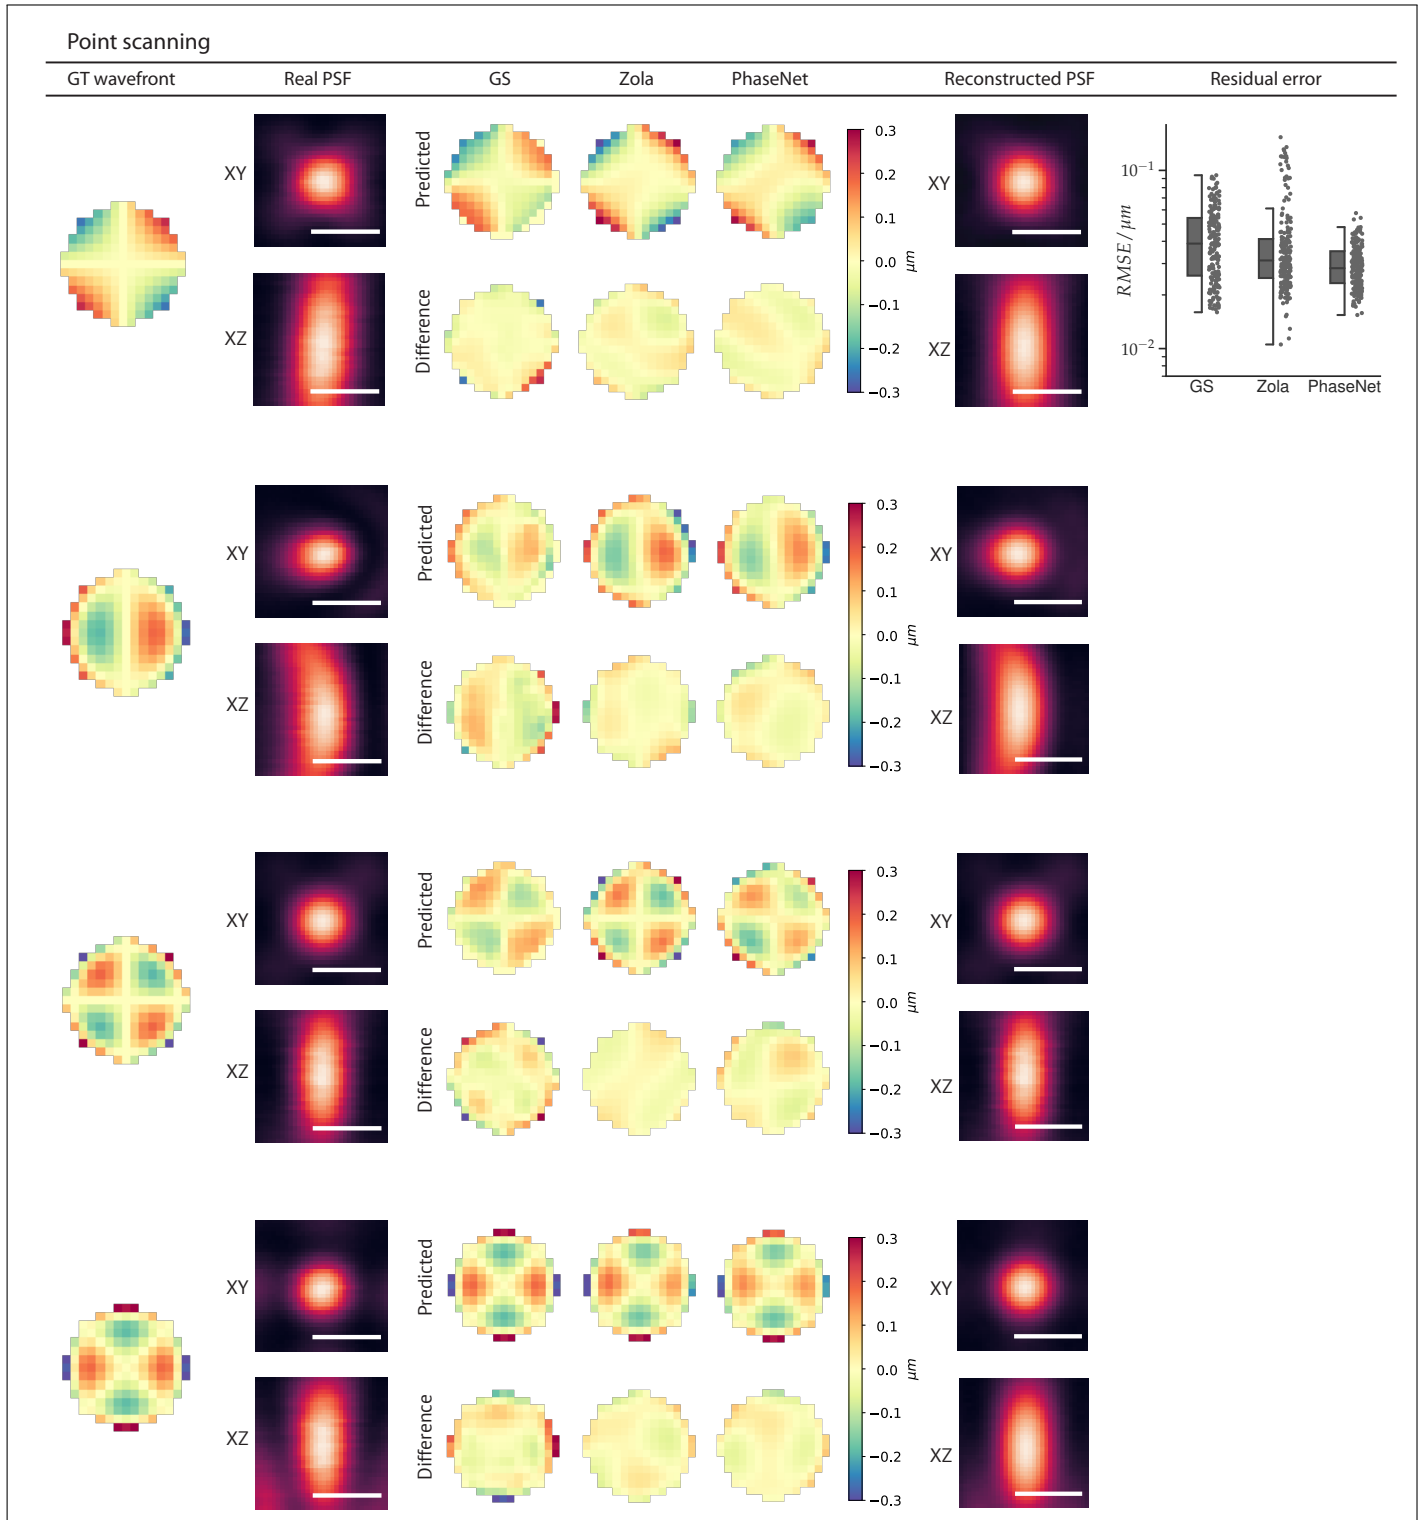

**Fig. S4.** Results of experimental single-mode aberrations for POINT SCANNING microscope set-up. A spatial light modulator was used to introduce single mode aberrations in the range  $[-0.11, 0.11]\mu\text{m}$  and the respective 3D stacks ( $n_z = 32$  planes) of  $80\text{ nm}$  gold beads were acquired. A network trained on synthetic PSFs was used for predicting aberration amplitudes ( $a_5, \dots, a_{15}$ ) from the 3D stacks. Here we show examples of the ground truth wavefront (reconstructed from the amplitudes of Zernike coefficients), lateral (XY) and axial (XZ) midplanes of the synthetic PSF, the wavefront estimated with Gerchberg-Saxton, Zola, and PHASENET (upper row) and their difference from the ground truth wavefront (lower row), and the reconstructed PSF from the PHASENET prediction. Additionally we show for all methods the error of the predicted wavefront (root mean square error, RMSE) for 198 PSFs. Scalebar:  $500\text{ nm}$ .

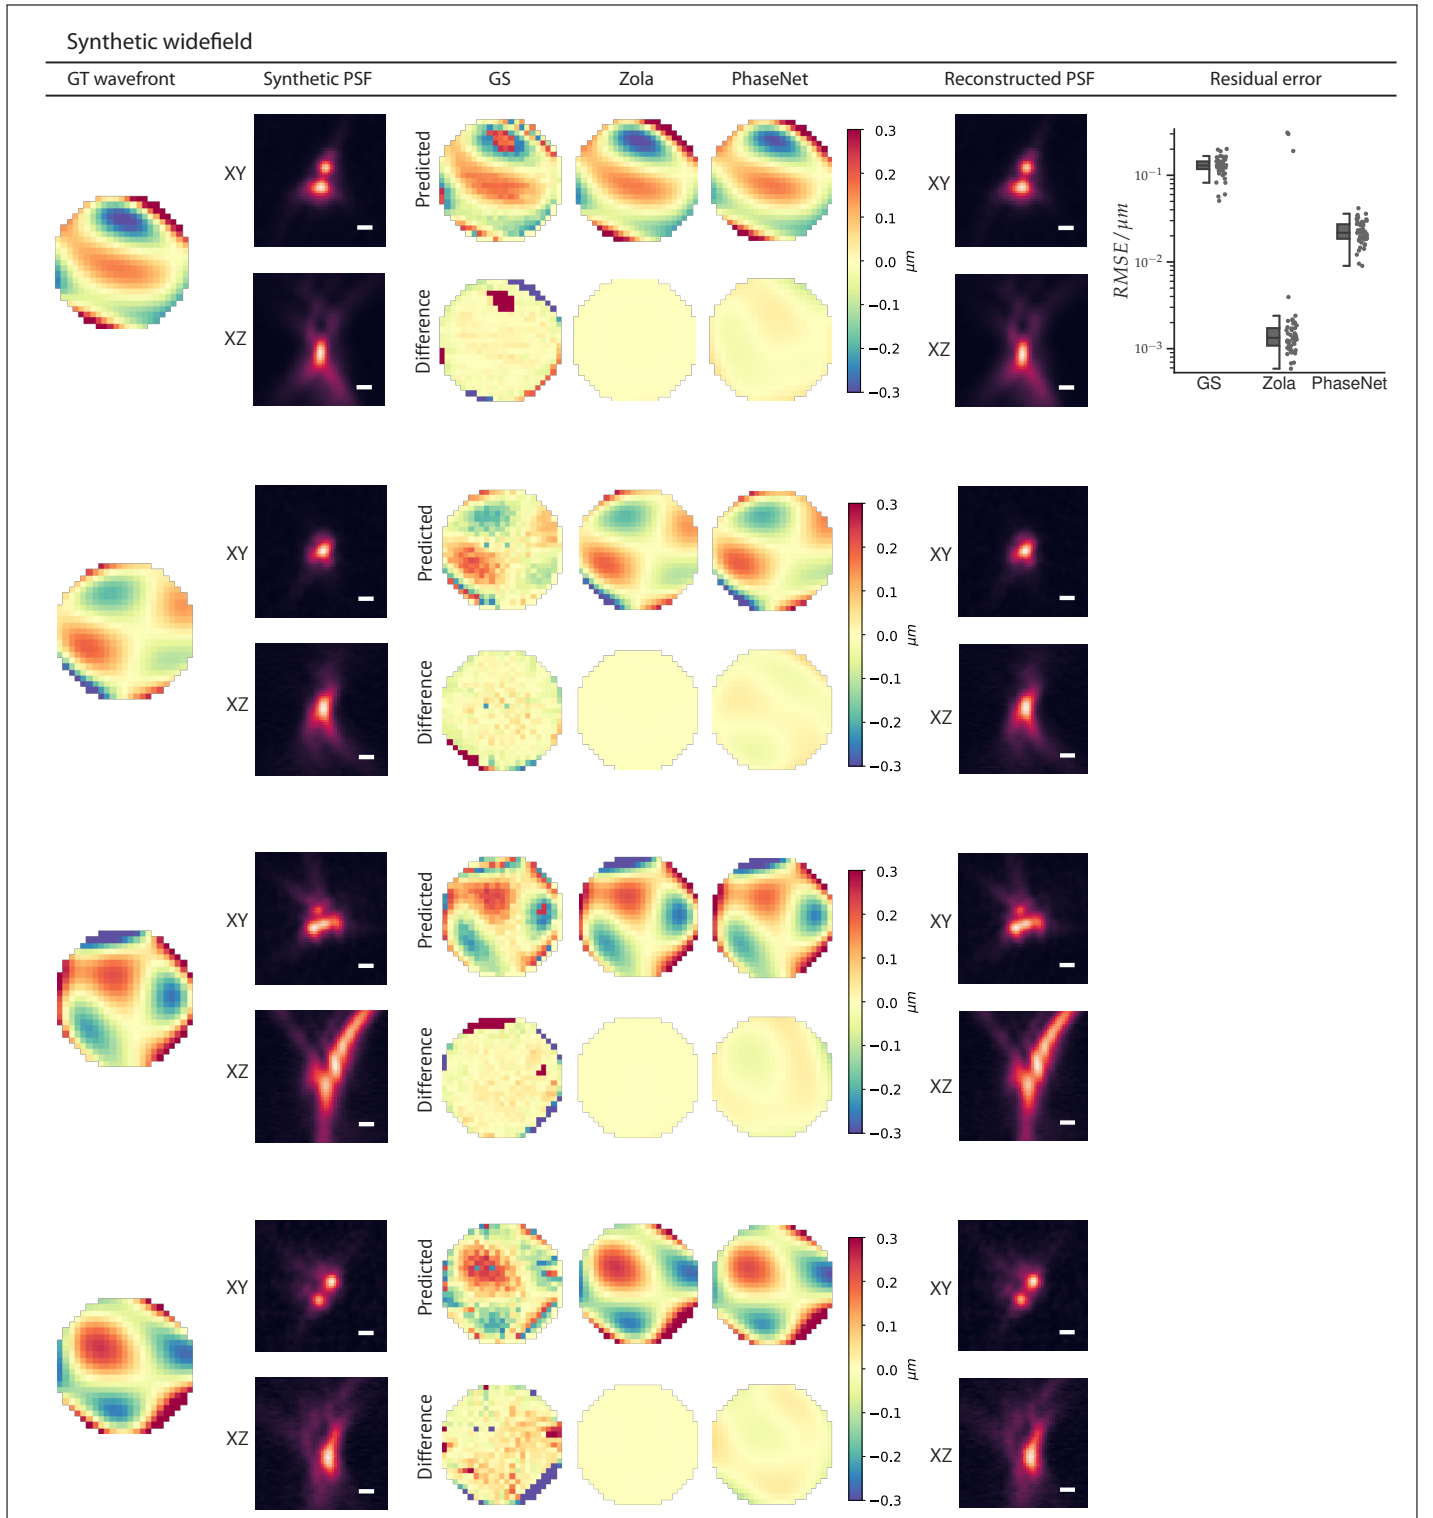

**Fig. S5.** Results on synthetic data. Random amplitudes of Zernike modes (Noll 5-15) in the range  $[-0.075, 0.075]\mu\text{m}$  for each mode was used to create GT wavefronts. The corresponding 3D intensity PSFs were simulated, convolved with a sphere of  $200\text{nm}$  diameter and noise was added to create a 3D synthetic PSFs. We cropped the PSFs to an isotropic volume of 50 planes and  $(50 \times 50)$  pixels to match the input shape of the network. Here we show examples of the ground truth wavefronts (reconstructed from the amplitudes of Zernike coefficients), lateral (XY) and axial (XZ) midplanes of the synthetic PSFs, the wavefronts estimated with Gerchberg-Saxton, Zola, and PHASENET (upper row) and their difference from the ground truth wavefronts (lower row), and the reconstructed PSFs from the PHASENET predictions. Additionally we show for all methods the error of the predicted wavefronts (root mean square error, RMSE) for 50 synthetic PSFs. Scalebar:  $500\text{nm}$ .

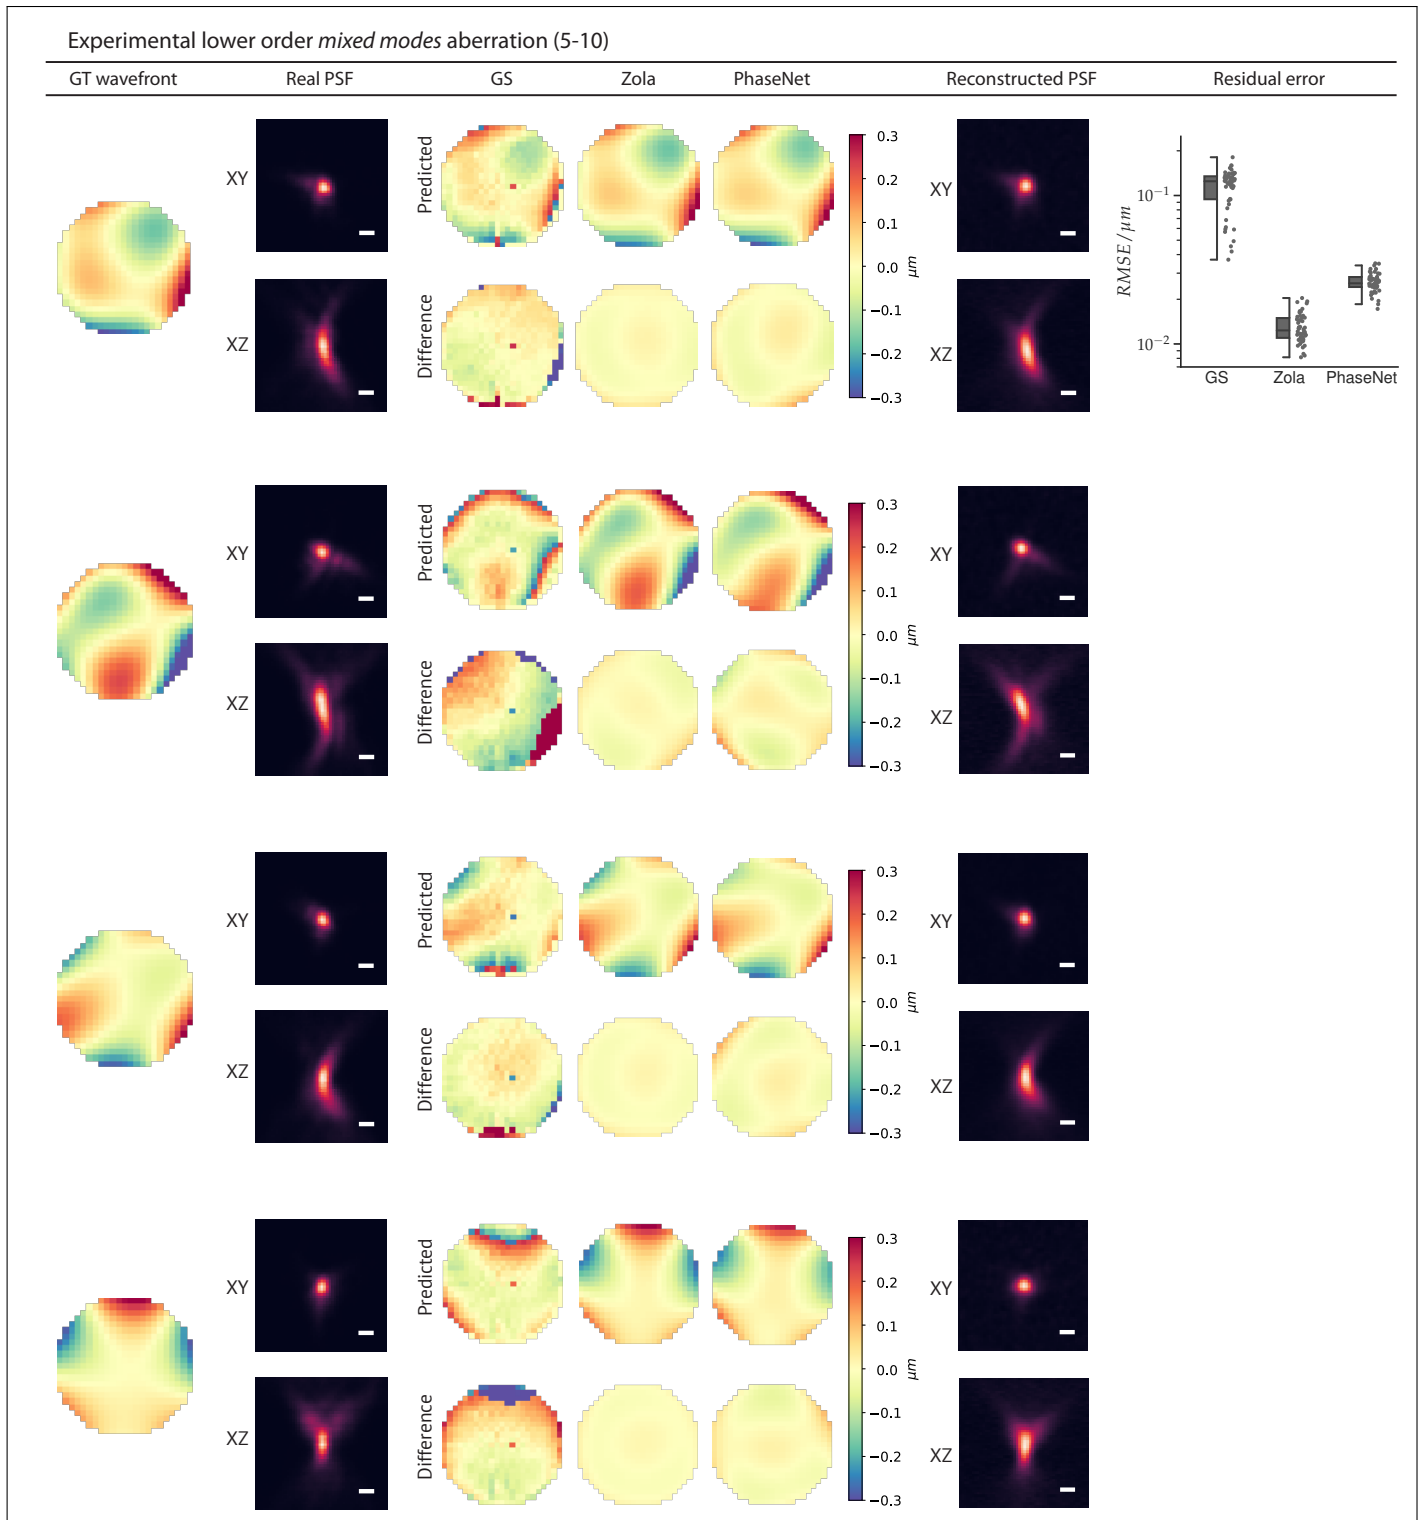

**Fig. S6.** Results of experimental low order *random modes* aberrations for widefield microscope set-up. A deformable mirror was used to introduce random amplitudes of low order modes (Noll 5-10) in the range  $[-0.075, 0.075] \mu\text{m}$  for each mode. Here we show additional examples for: the ground truth wavefront (reconstructed from the amplitudes of Zernike coefficients), lateral (XY) and axial (XZ) midplanes of the acquired bead (PSF) stacks, the wavefront estimated with Gerchberg-Saxton, Zola, and PHASENET (upper row) and their difference from the ground truth wavefront (lower row), and the reconstructed PSF from the PHASENET prediction. Additionally we show for all methods the error of the predicted wavefront (root mean square error, RMSE) for 50 PSFs. Scalebar: 500 nm.

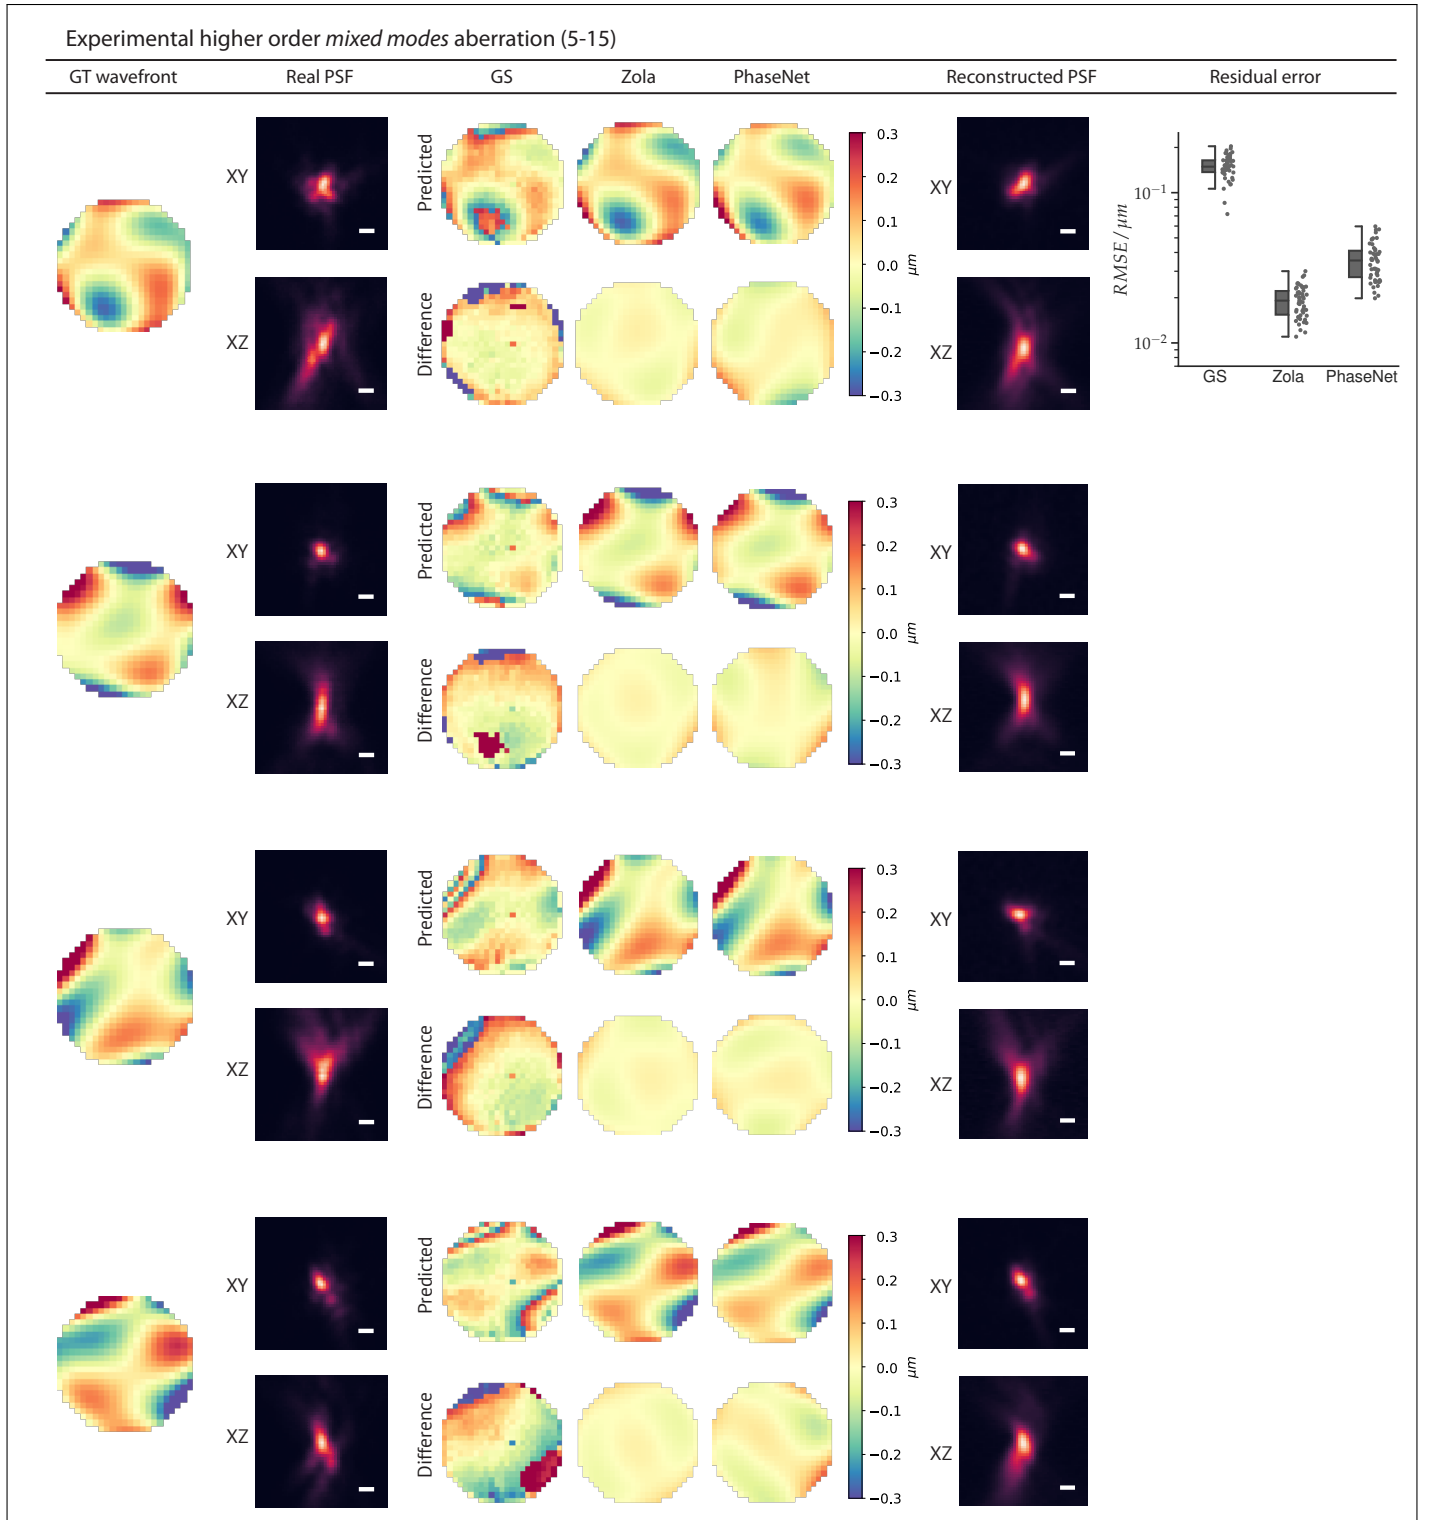

**Fig. S7.** Results of experimental high order *random modes* aberrations for widefield microscope set-up. A deformable mirror was used to introduce random amplitudes of low order modes (Noll 5-15) in the range  $[-0.075, 0.075]\mu\text{m}$  for each mode. Here we show additional examples for: the ground truth wavefront (reconstructed from the amplitudes of Zernike coefficients), lateral (XY) and axial (XZ) midplanes of the acquired bead (PSF) stacks, the wavefront estimated with Gerchberg-Saxton, Zola, and PHASENET (upper row) and their difference from the ground truth wavefront (lower row), and the reconstructed PSF from the PHASENET prediction. Additionally we show for all methods the error of the predicted wavefront (root mean square error, RMSE) for 50 PSFs. Scalebar: 500 nm.
